# Supplementary material for: Decoding the human brain tissue response to radiofrequency excitation using a biophysical-model-free deep MRI on a chip framework
Source: arXiv:2408.08376 ancillary file (2024-08-19)
Supplement: Supplementary file 1 [file supporting_figures.pdf]

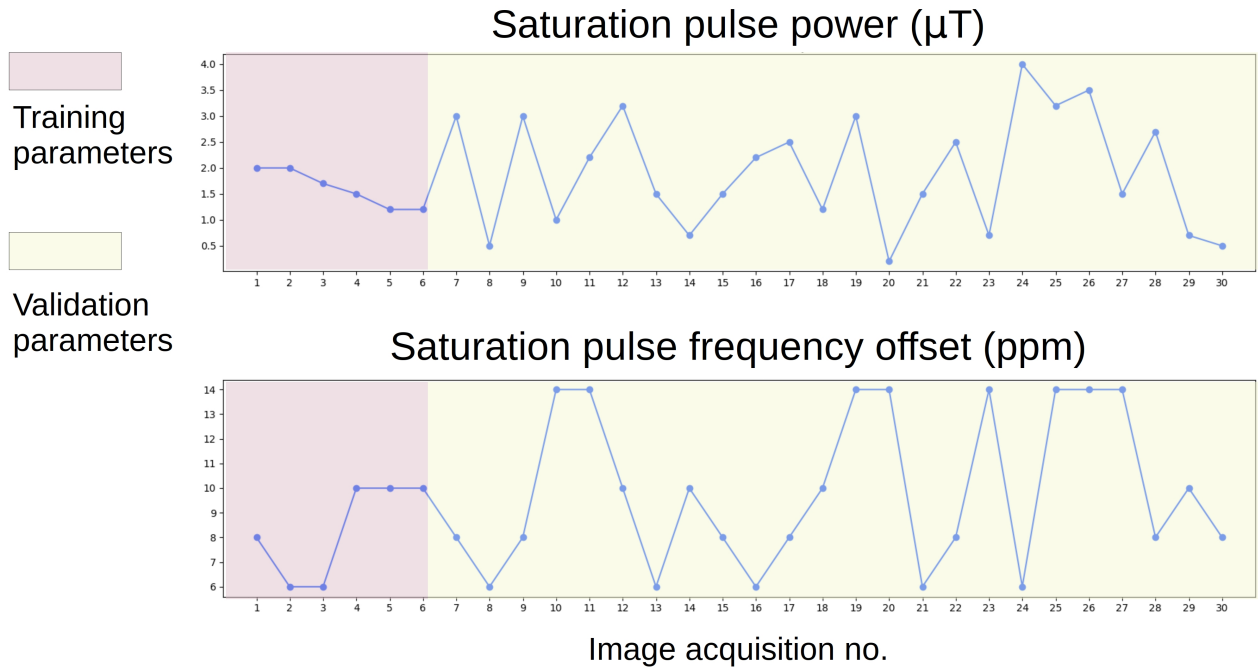

**Supporting Information Figure S1.** Pseudo-random MRI acquisition protocol used for training and validating the core module. The first six images were acquired according to the saturation pulse power and frequency offset patterns in the pink region, and served as per-subject calibration data. The remaining 24 images (yellow region pattern) were automatically predicted by DeepMonC. The same acquisition pulse power pattern was used for the semisolid MT and amide CEST protocols, but with the frequency offset fixed at 3.5 ppm (downfield of water) for amide CEST<sup>26</sup>.

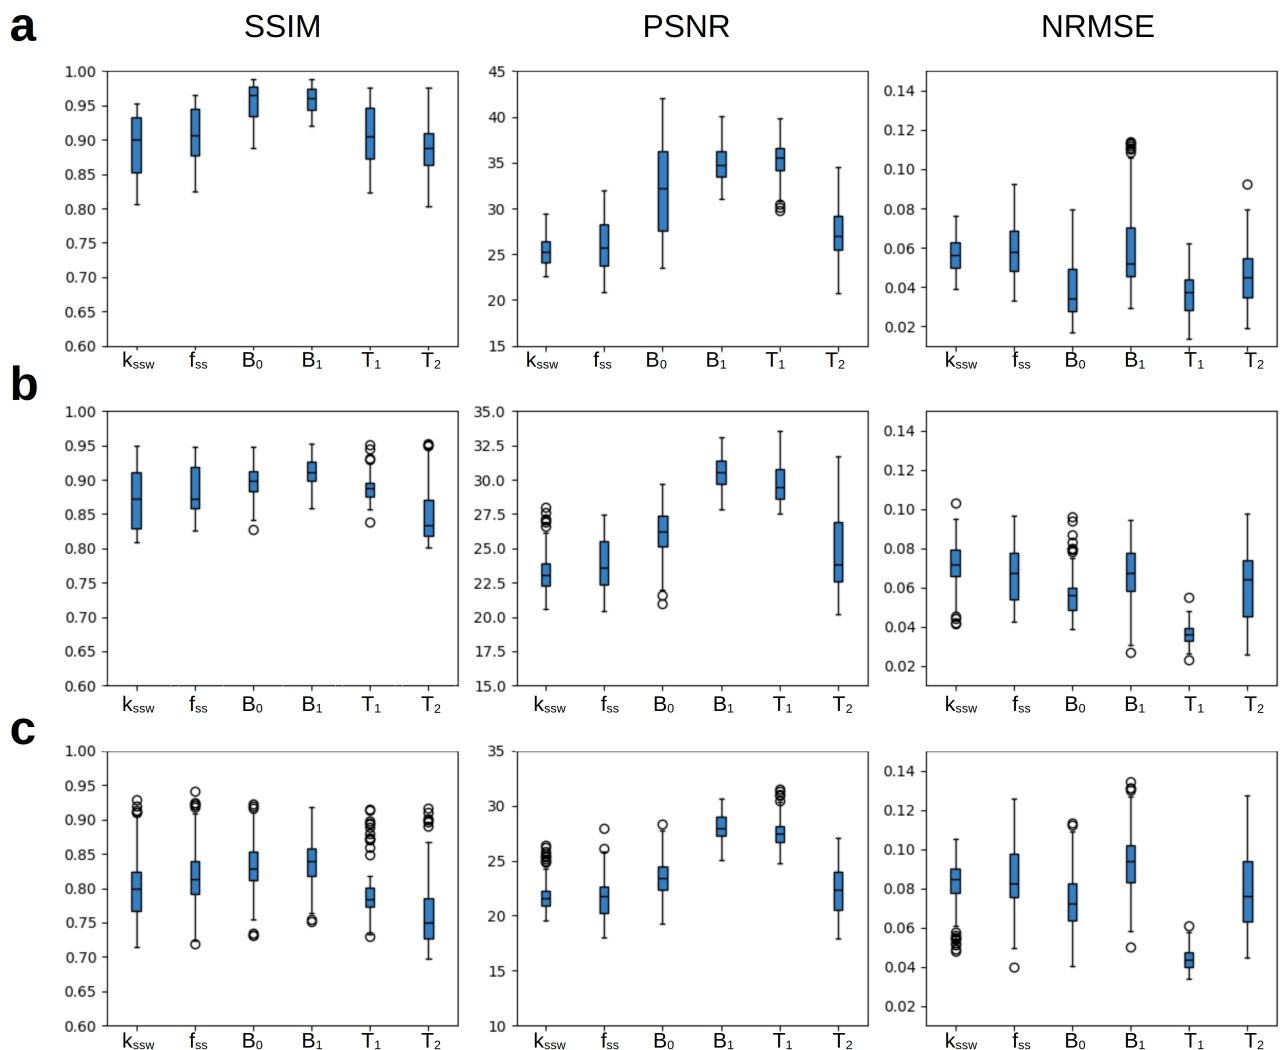

**Supporting Information Fig. S2.** Performance analysis using the SSIM, PSNR and NRMSE metrics for the quantification task (**Fig. 1b**). Six calibration images and their acquisition parameter counterparts served as input for the quantification module and six quantitative parameter maps were generated automatically.  $f_{SS}$  - semisolid MT proton volume fraction;  $k_{SSW}$  - semisolid MT proton exchange rate;  $T_1$  - water longitudinal relaxation time;  $T_2$  - water transverse relaxation  $B_0$  - static magnetic field;  $B_1$  - transmit magnetic field.

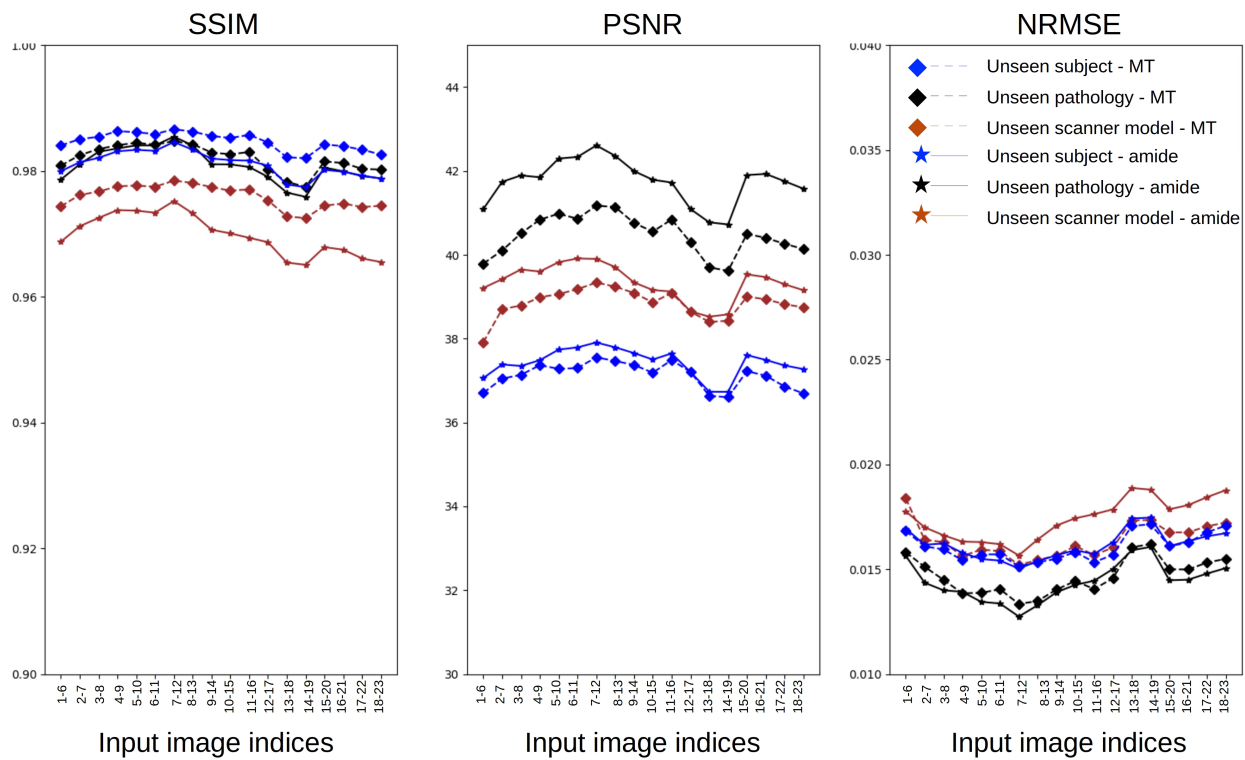

**Supporting Information Fig. S3.** DeepMonC on-demand contrast generation performance, with respect to various sets of calibration images and desired output contrasts. Eighteen different combinations were evaluated (input image indices are described across the x-axis, referring to the acquisition parameters described in Supporting Information Figure S1).

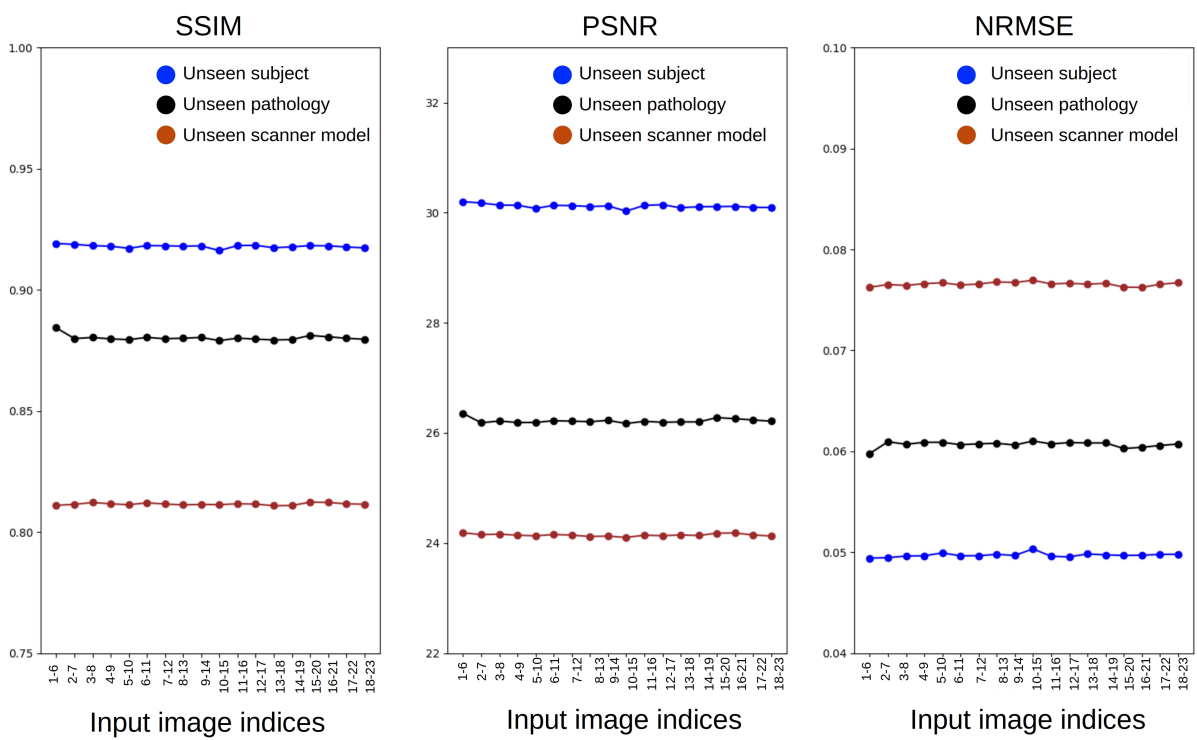

**Supporting Information Fig. S4.** DeepMonC quantification module performance with respect to various sets of calibration images. Eighteen different combinations were evaluated (input image indices are described across the x-axis, referring to the acquisition parameters described in Supporting Information Figure S1).

**Supporting Information Movie M1. Automatic prediction of multi-contrast semisolid MT-weighted images.** A comparison between representative ground truth (**top**) and DeepMonC-predicted (**bottom**) images across the entire 3D human brain (three orientations are shown).

**Supporting Information Movie M2. Automatic prediction of multi-contrast amide proton transfer CEST-weighted images.** A comparison between representative ground truth (**top**) and DeepMonC-predicted (**bottom**) images across the entire 3D human brain (three orientations are shown).

**Supporting Information Movie M3. Recursive prediction of semisolid MT-weighted images.** After a rapid pre-calibration with 6 images (acquired within 28.2 s), 24 new multi-contrast images are predicted (**left**) according to on-demand acquisition protocol parameters (**right**).

**Supporting Information Movie M4. Recursive prediction of amide proton transfer CEST-weighted images.** After a rapid pre-calibration with 6 images (acquired within 28.2 s), 24 new multi-contrast images are predicted (**left**) according to on-demand acquisition protocol parameters (**right**).
